# Supplementary material for: Exploring the Landscape of effective field theories
Source: arXiv:1912.08935 source file (2023-03-17)
Supplement: Supplementary file 1 [file App_Open_String_Moduli.tex]

\chapter{An introduction to Open String Moduli}
\label{app:Open}
